# Supplementary material for: The Opaque Heart of the Galaxy IC 860: Analogous Protostellar, Kinematics, Morphology, and Chemistry
Source: arXiv:2210.04499 source file (2023-01-03)
Supplement: Supplementary file 1 [file appendix.tex]

\begin{appendix}

\section{Principal Components and Eigenvectors}

Figs \ref{fig:PC1-3} and \ref{fig:PC4-6} show the tomograms and eigenvectors of IC~860. 

\begin{figure*}
    \centering
    \includegraphics[width=0.9\textwidth]{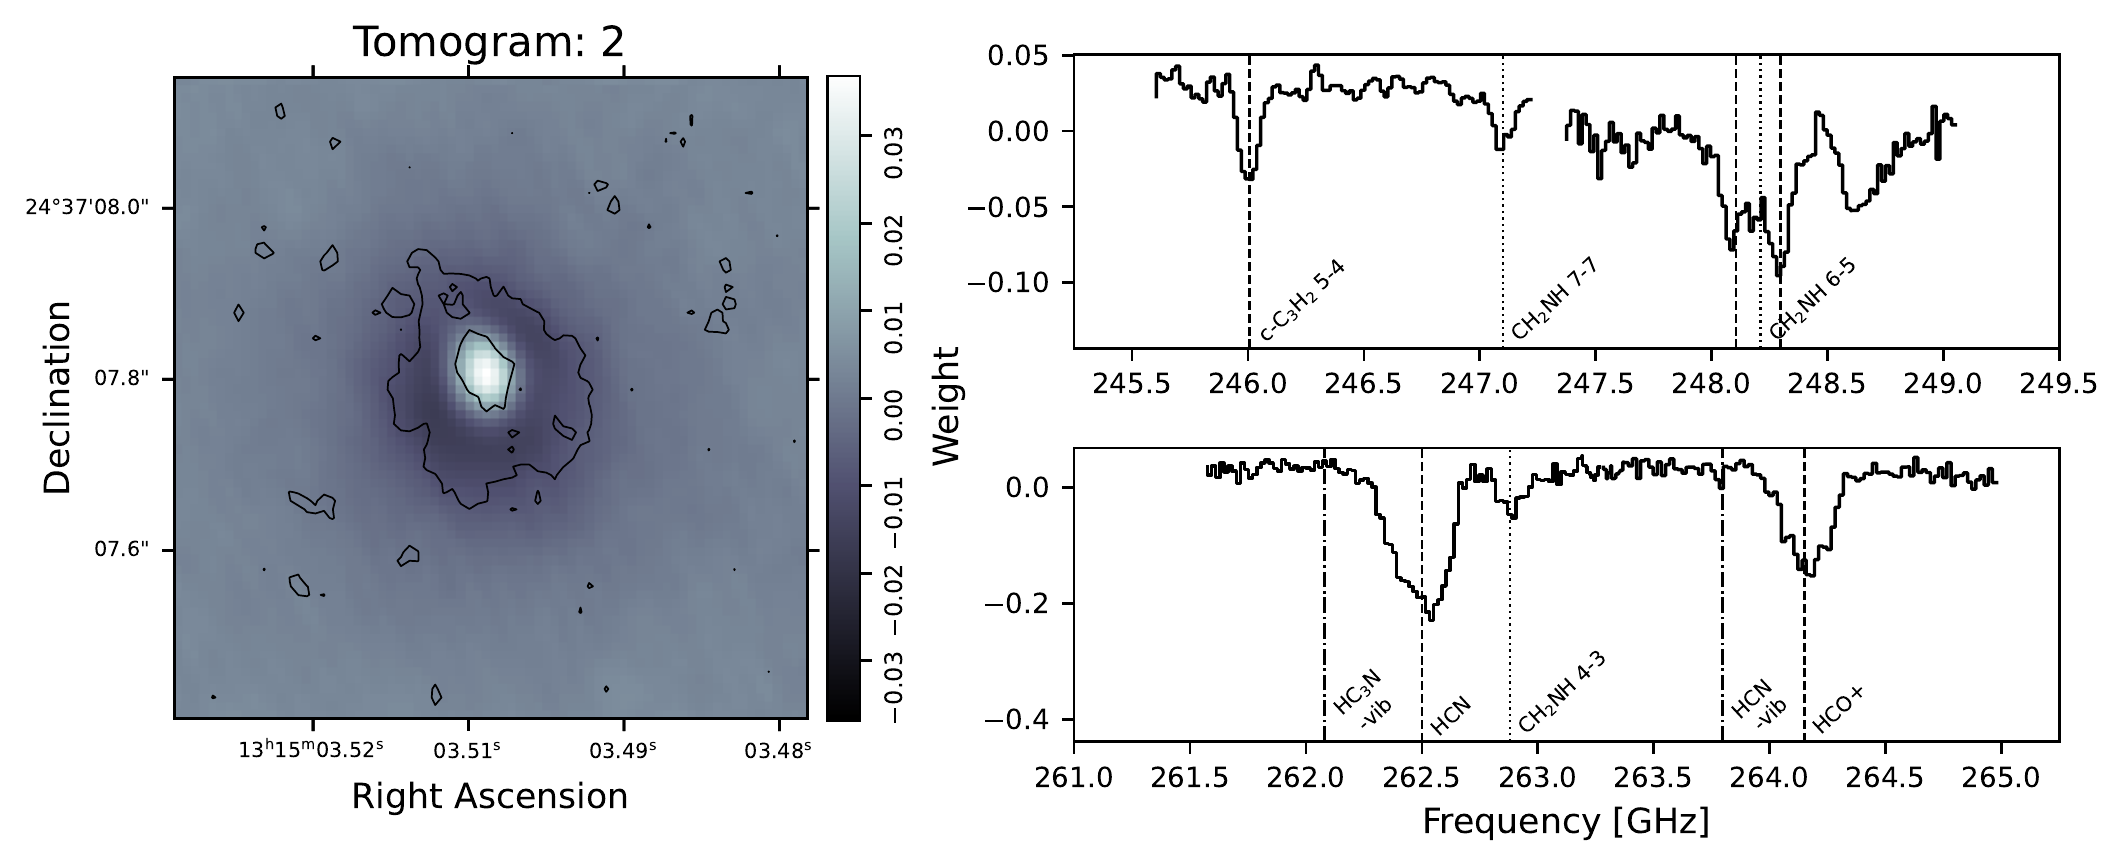}
    \includegraphics[width=0.9\textwidth]{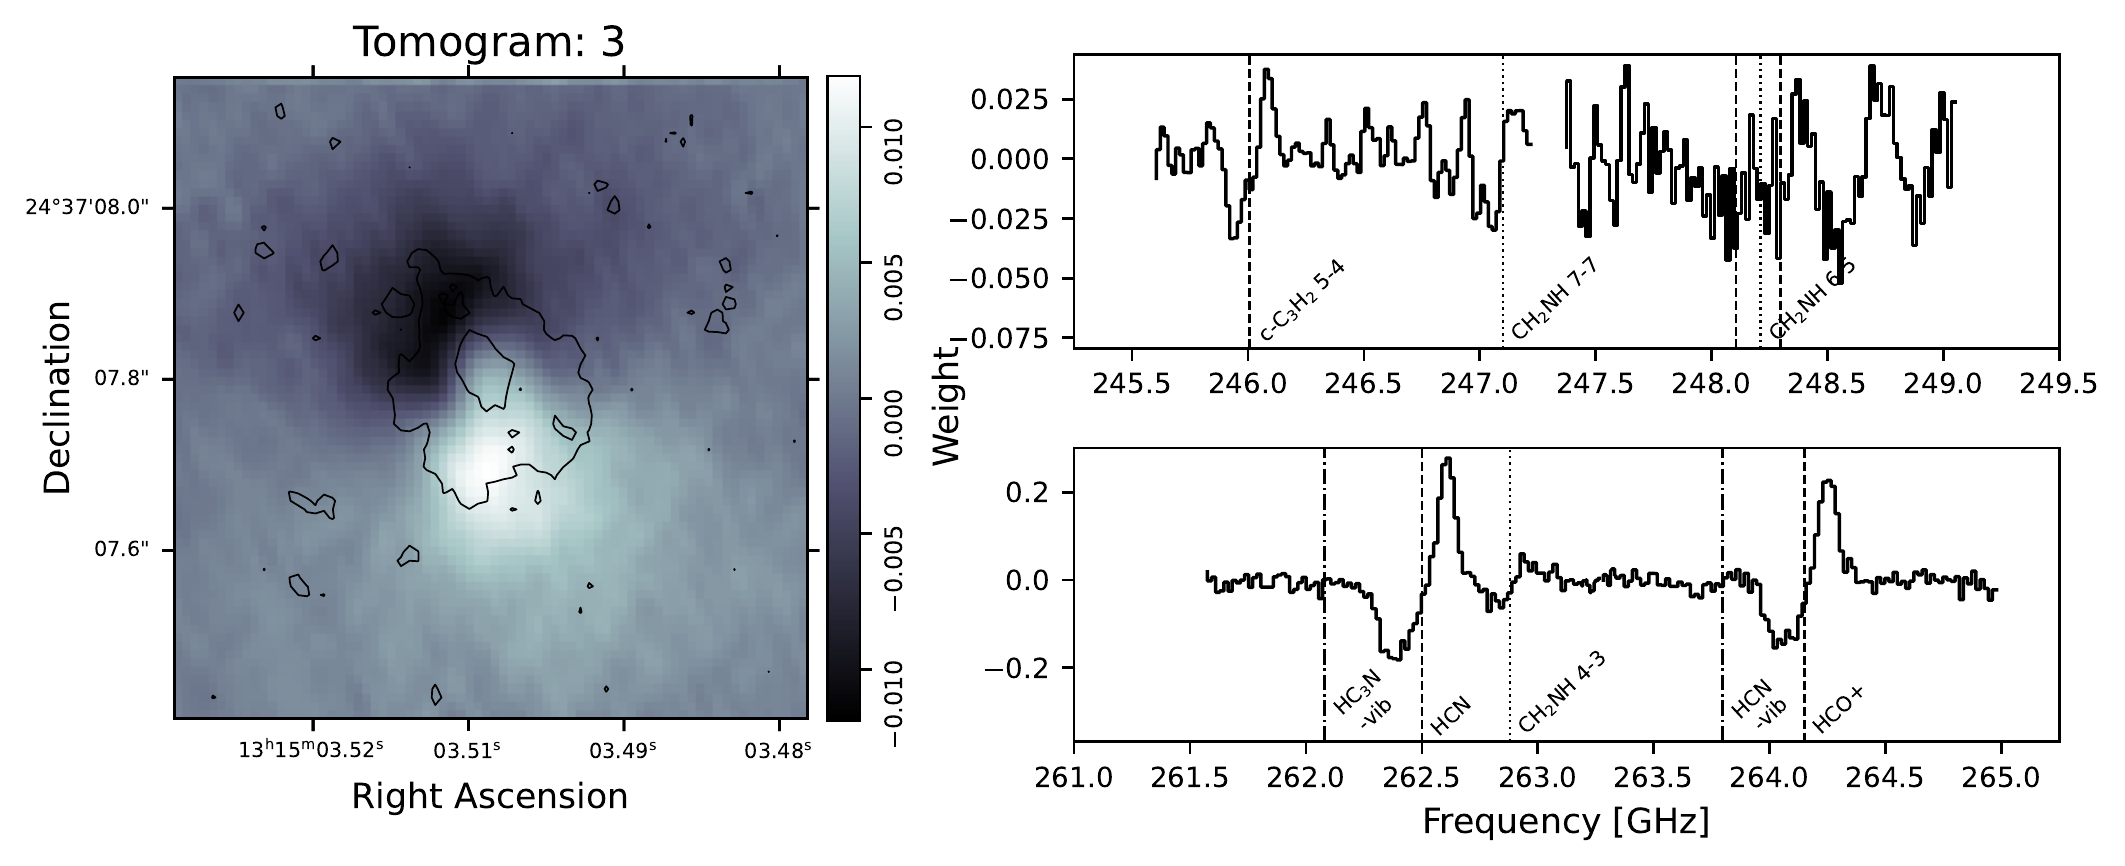}
    \caption{Principal Components two and three. White means stronger correlation and black means anti-correlation. 
    The 3$\sigma$ contour of the CH$_2$NH $4_{13}$-$3_{12}$ transition is plotted in black.
    PC 2 shows evidence for an ``envelope'' around the mm continuum, and PC~shows anti-correlated red and blueshifted emission indicative of rotation.
    The vertical lines mark the redshifted rest frequencies of the same lines identified in Figure \ref{fig:PC0}.
    }
    \label{fig:PC1-3}
\end{figure*}

\begin{figure*}
    \centering
    \includegraphics[width=0.95\textwidth]{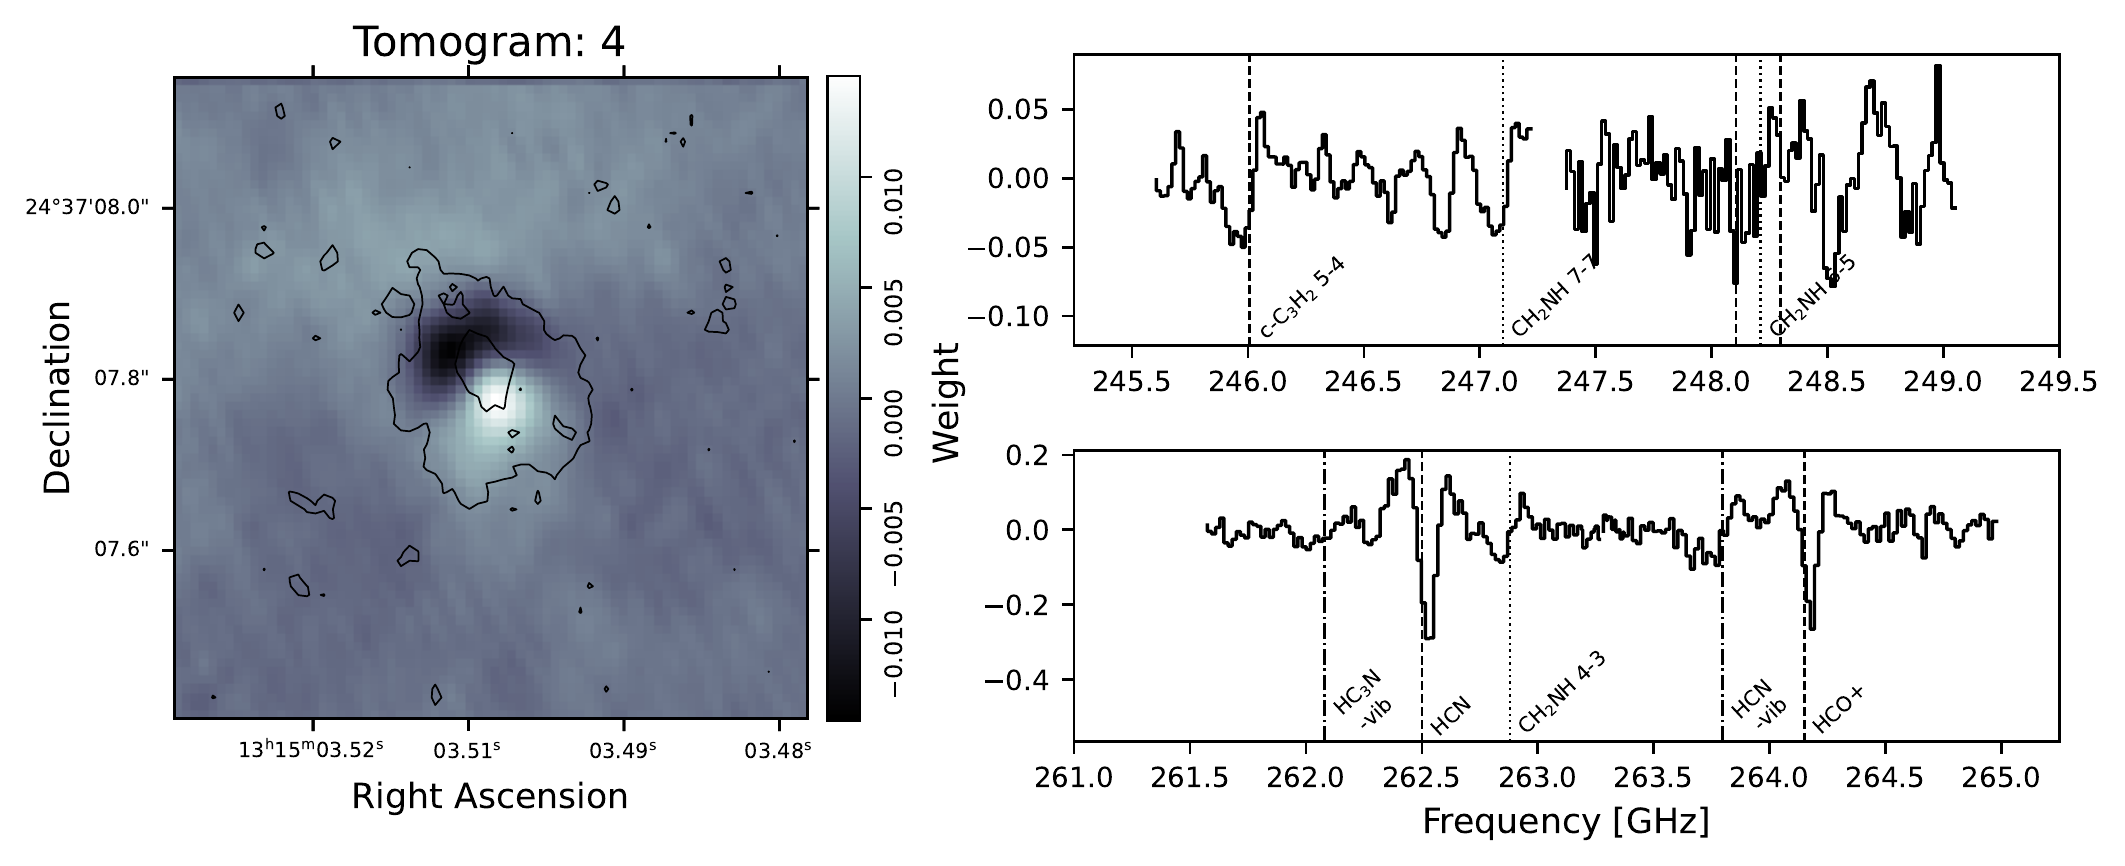}
    \includegraphics[width=0.95\textwidth]{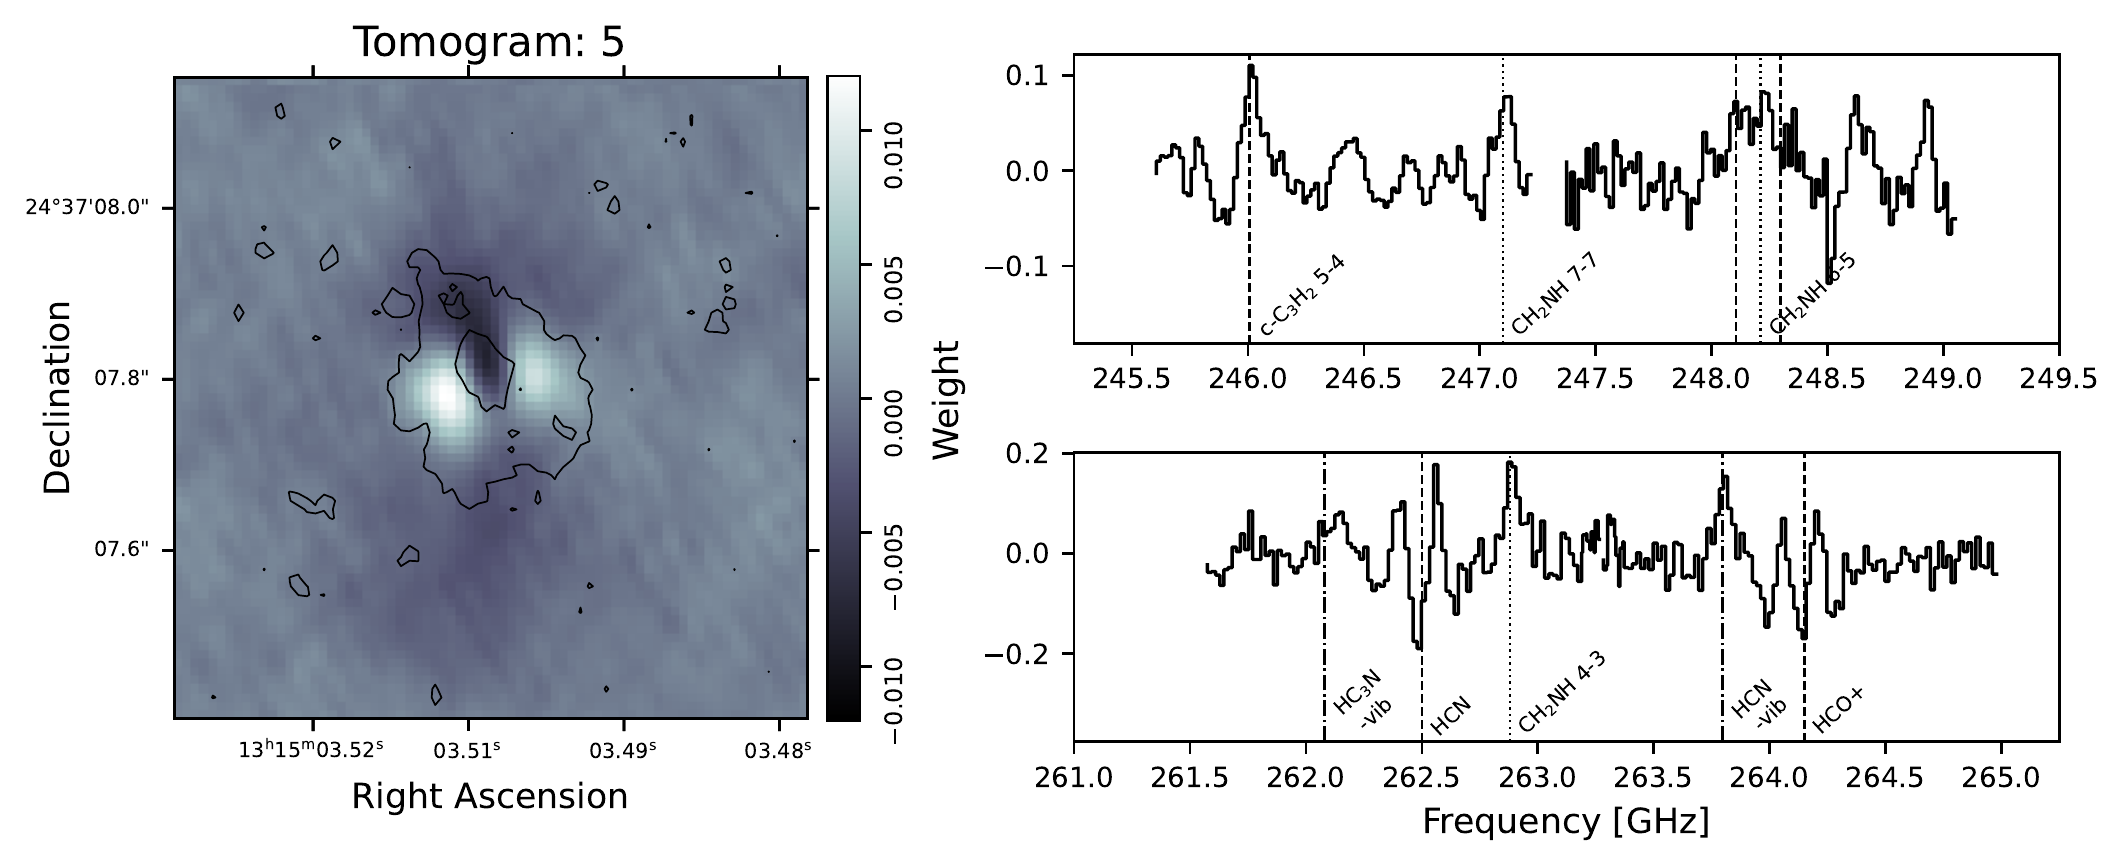}
    \includegraphics[width=0.95\textwidth]{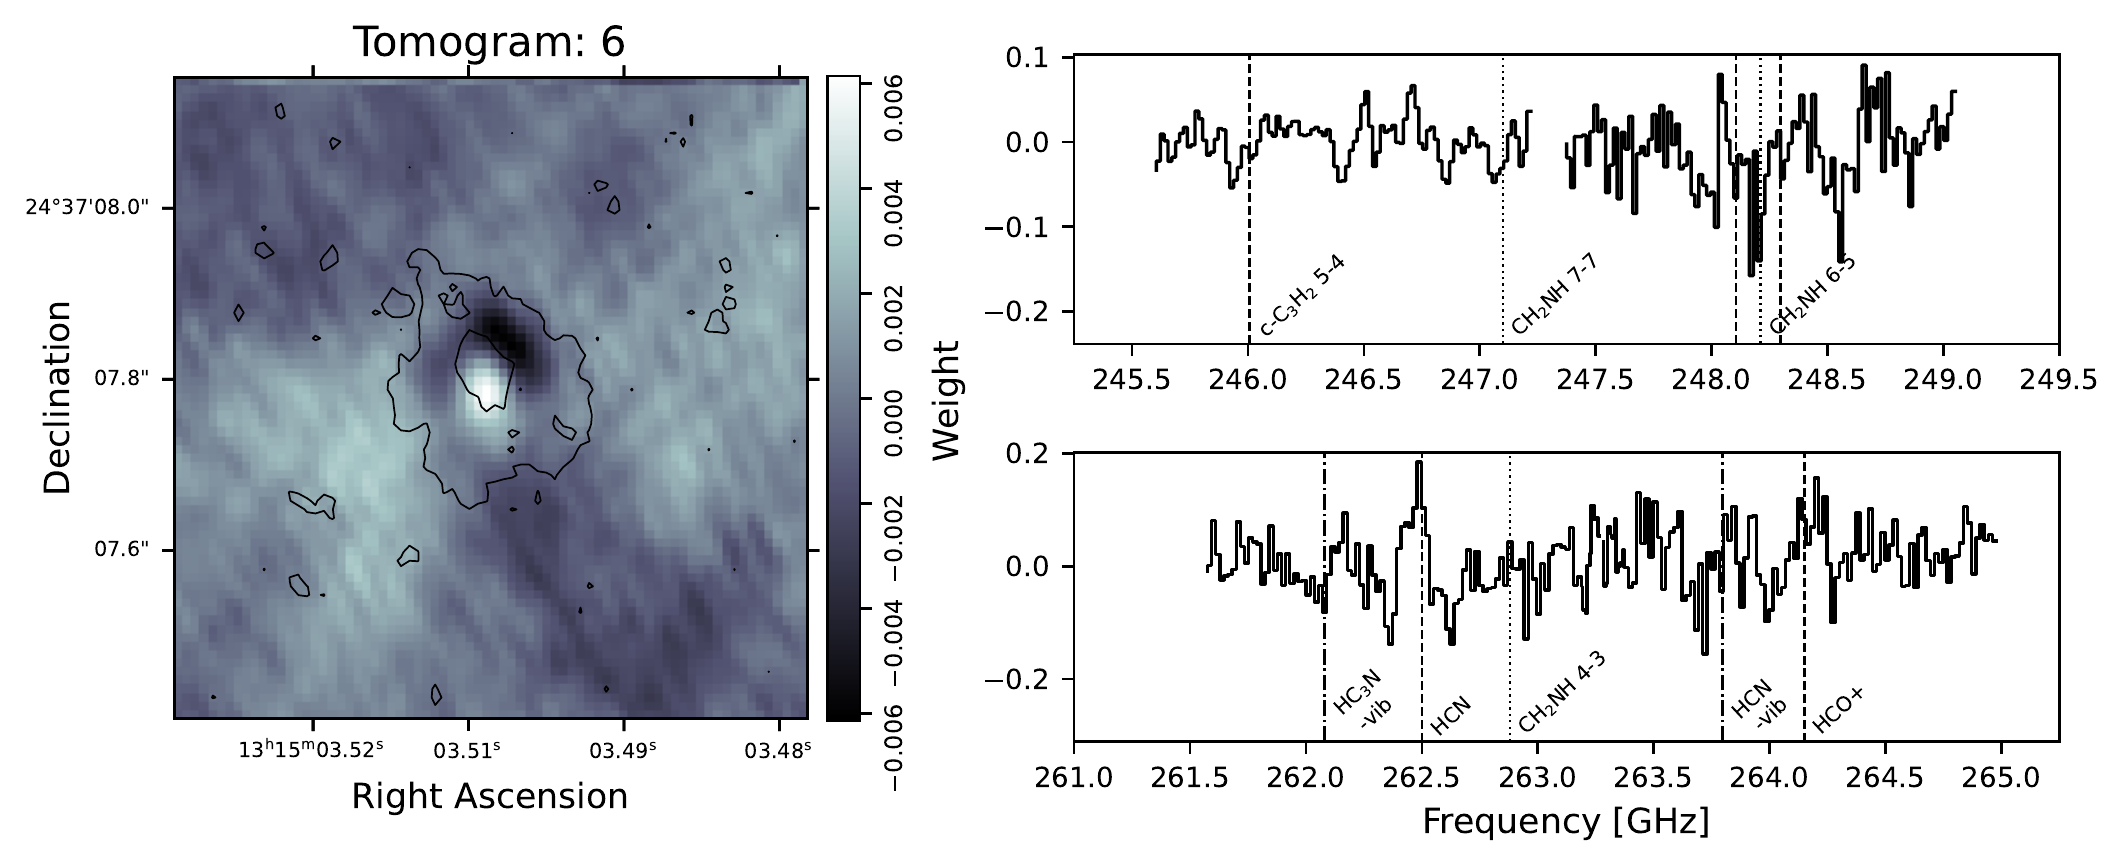}
    \caption{Principal Components four to six. White means stronger correlation and black means anti-correlation. 
    The 3$\sigma$ contour of the CH$_2$NH $4_{13}$-$3_{12}$ transition is plotted in black.
    PC~4 shows anti-correlation between red and blue shifted vibrational transitions, indicating slower rotating structure and a change in excitation of the molecular gas. 
    PC~5 shows a double lobed structure associated with line wings.
    PC~6 shows correlation with the low velocity components of the ground state HCN line and weak anti-correlation with the line wings. 
    The vertical lines mark the redshifted rest frequencies of the same lines identified in Figure \ref{fig:PC0}.
    }
    \label{fig:PC4-6}
\end{figure*}

\section{PCA Enhanced Data Cubes}

Figs \ref{fig:PCAE-HCN} and \ref{fig:PCAE-HCO+} show the channel maps of the original calibrated data cube, the PCA enhanced data cube, and the continuum subtracted data cube.

\begin{figure*}
    \centering
    \includegraphics[width=0.95\textwidth]{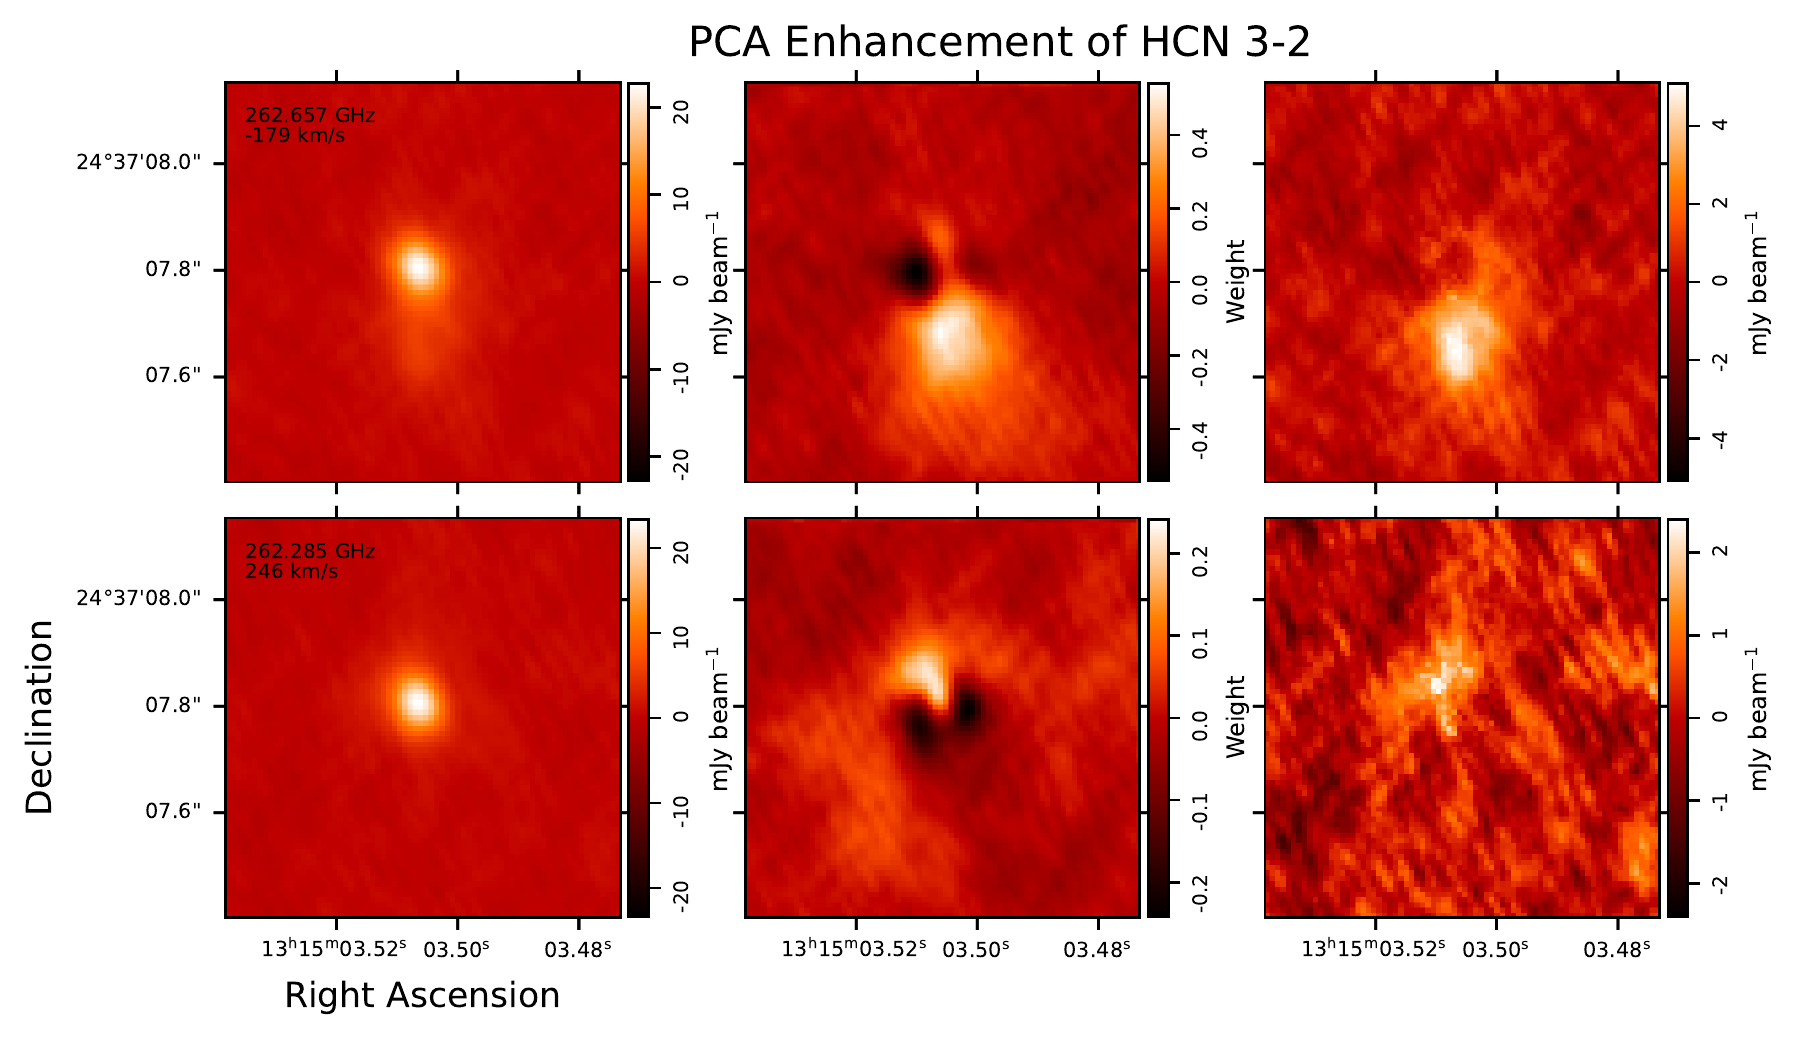}
    \caption{Comparison between the original data cube, the PCA enhanced cube, and the continuum subtracted data cube.
     The left column displays the original data cube, the center column the PCA enhanced cube, and the right column the continuum subtracted cube.
    The top row of panels shows the 262.657~GHz channel corresponding to -179~\kms  of the HCN~(4-3) transition, adopting a redshift of 0.0129 for IC~860. 
    The bottom row of panels shows the 262.285~GHz 246~\kms channel.
    The center image is given in weight and not in mJy~beam$^{-1}$ as with the other two panels.
    }
    \label{fig:PCAE-HCN}
\end{figure*}

\begin{figure*}
    \centering
    \includegraphics[width=0.95\textwidth]{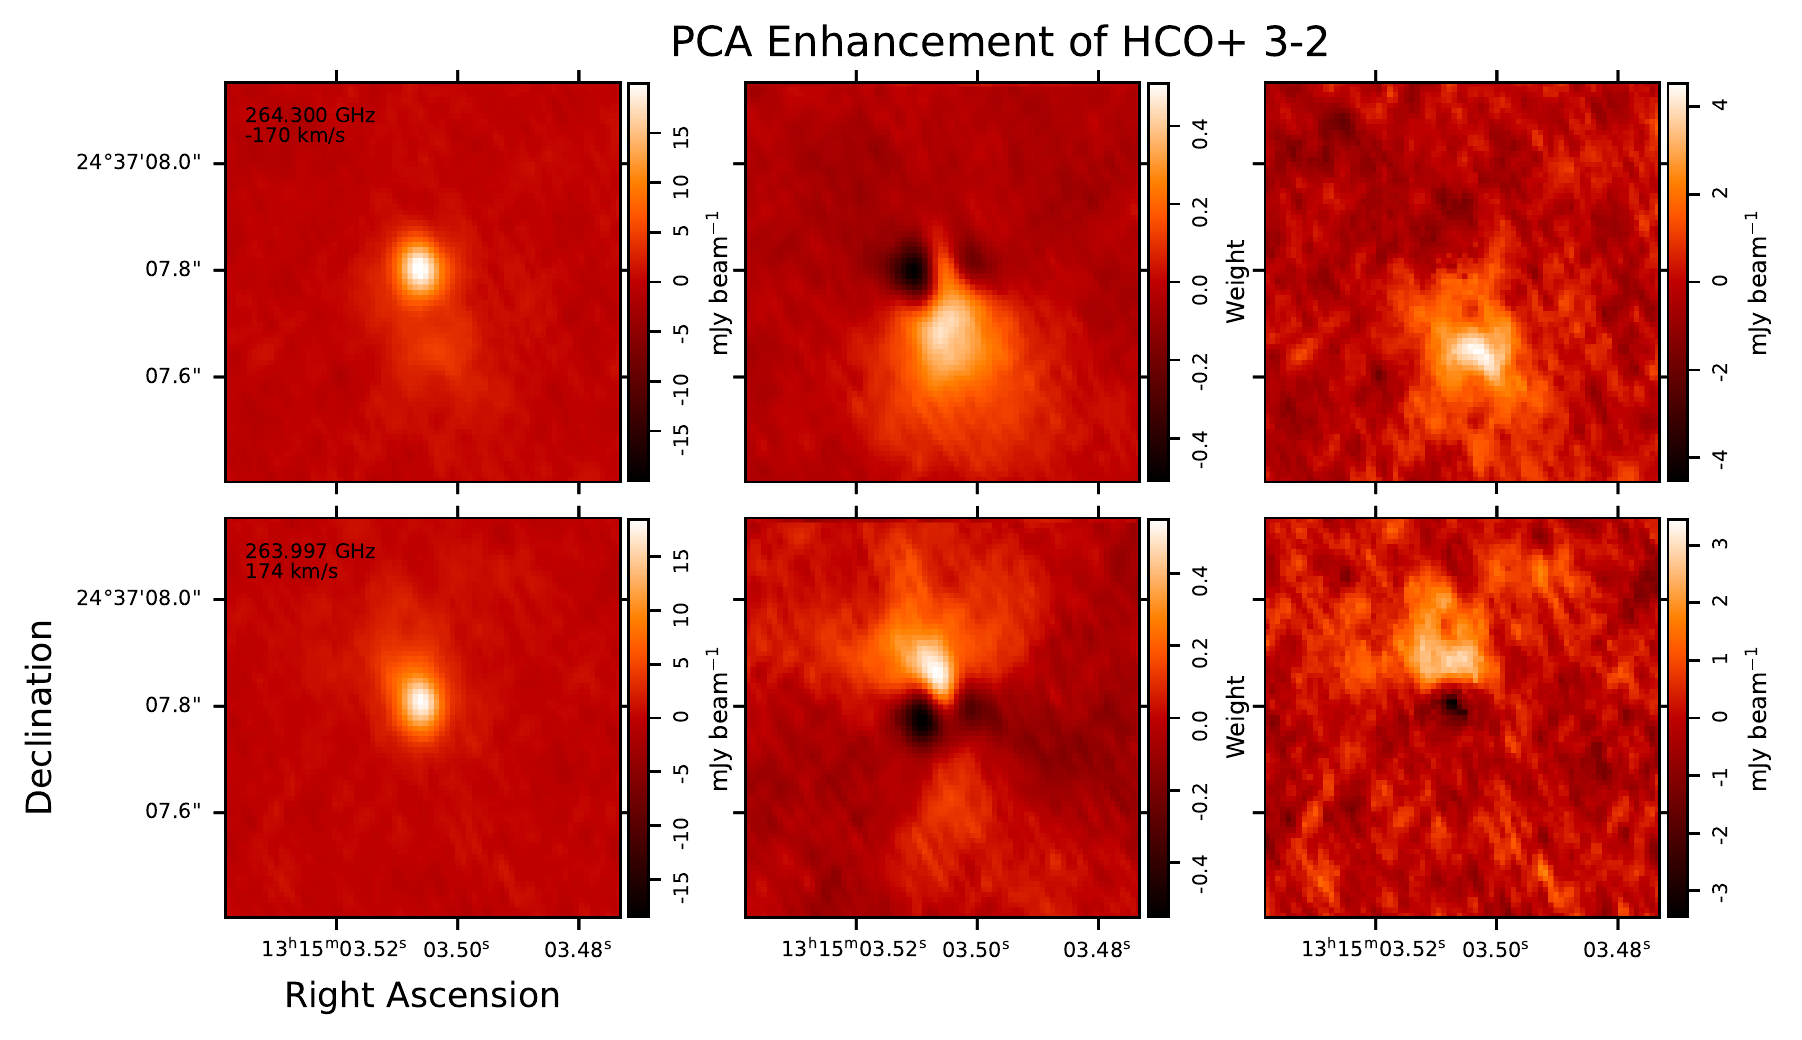}
    \caption{Comparison between the original data cube, the PCA enhanced cube, and the continuum subtracted data cube.
     The left column displays the original data cube, the center column the PCA enhanced cube, and the right column the continuum subtracted cube.
    The top row of panels shows the 264.318~GHz channel corresponding to -191~\kms  of the HCN~(4-3) transition, adopting a redshift of 0.0129 for IC~860. 
    The bottom row of panels shows the 263.979~GHz 194~\kms channel.
    The center image is given in weight and not in mJy~beam$^{-1}$ as with the other two panels.
    }
    \label{fig:PCAE-HCO+}
\end{figure*}

\end{appendix}
